# Supplementary material for: Discriminative Clustering with Representation Learning with any Ratio of Labeled to Unlabeled Data
Source: arXiv:1912.12979 source file (2023-02-17)
Supplement: Supplementary file 1 [file appendix4_additional_results.tex]

%\section{Additional Experimental Results}
%\label{app:additional_results}
%In this appendix we present additional experimental results that expand upon those presented in Section~\ref{sec:experiments}.
%

%\paragraph{Visualization of feature representations.} Figure~\ref{fig:mnist50_viz} visualizes the feature representations of unlabeled MNIST digits at different points in the training process. In each case the features were projected to 2-D with the Scikit-Learn \citep{pedregosa2011} implementation of t-SNE \citep{vandermaaten2008}. Based on these t-SNE representations, the plots were then produced. The code to produce the plots was adapted from Andrej Karpathy's Matlab code.\footnote{\url{https://cs.stanford.edu/people/karpathy/cnnembed/}} It first scales the t-SNE representations so they all lie in $[0,1]^2$ and creates an evenly-spaced $40\times40$ grid over $[0,1]^2$. Then, for each square in the grid, it checks whether any image's t-SNE representation lies in that square. If any such images exist, it chooses one at random and displays the original image in that square. The images are then color-coded according to the ground-truth labels.
%
%\def\tsnewidth{1.0}
%\begin{figure}[t!]
%\vspace{-0.2cm}
%\begin{subfigure}{.49\columnwidth}
%\includegraphics[width=\tsnewidth\columnwidth]{figures/mnist/mnist_cluster_plot_4096_5_restart_iter_-1_tsne_color.pdf}
%\caption{\label{fig:tsne_raw}Raw}
%\end{subfigure}\hfill
%\begin{subfigure}{.49\columnwidth}
%\includegraphics[width=\tsnewidth\columnwidth]{figures/mnist/mnist_cluster_plot_4096_80_restart_iter_0_tsne_color.pdf}
%\caption{\label{fig:tsne_unsup} Unsupervised initialization}
%\end{subfigure}
%\begin{subfigure}{.49\columnwidth}
%\vspace{0.4cm}
%\includegraphics[width=\tsnewidth\columnwidth]{figures/mnist/mnist_cluster_plot_4096_100_restart_iter_100_2020-08.pdf}
%\caption{\label{fig:tsne_sup} Supervised initialization}
%\end{subfigure}\hfill
%\begin{subfigure}{.49\columnwidth}
%\vspace{0.4cm}
%\includegraphics[width=\tsnewidth\columnwidth]{figures/mnist/mnist_cluster_plot_4096_50_restart_iter_500_2020-08.pdf}
%\caption{\label{fig:tsne_xsdc} XSDC}
%\end{subfigure}
%\caption{\label{fig:mnist50_viz} Visualizations of the unlabeled MNIST features obtained when training the LeNet-5 CKN with 50 labeled observations (where applicable). The CKN features were projected to 2-D using t-SNE. The features were obtained at different stages, as indicated in the sub-captions.}
%\end{figure}
%
%The batch size used to produce the t-SNE representations and the corresponding plots was 4096. The default parameters were used for generating the t-SNE representations. We created each plot with 20 random initializations and present the ones that visually appeared to be the best.
%
%Figure~\ref{fig:tsne_raw} visualizes the raw digits. By ``raw'' we mean that the digits were not input into the network; they were only standardized before applying t-SNE. Comparing this figure with Figure~\ref{fig:tsne_unsup}, which visualizes the feature representations from the network with randomly initialized filters, we can see that in both plots the 4's and 9's are mixed together. Furthermore, the 5's are split into two parts in Figure~\ref{fig:tsne_raw}. Figure~\ref{fig:tsne_sup} depicts the feature representations after the supervised initialization. Figure~\ref{fig:tsne_sup} is similar to \ref{fig:tsne_unsup}, although the 3's and 8's are a bit more separated. Finally, Figure~\ref{fig:tsne_xsdc} depicts the features representations after running XSDC. Comparing Figures \ref{fig:tsne_sup} and \ref{fig:tsne_xsdc}, we can see that XSDC tends to separate the clusters more relative to the supervised initialization. While the 3's, 5's, and 8's are generally better separated after running XSDC, the 4's and 9's are still mixed together.

%\paragraph{Effect of additional constraints.} Next, Figure~\ref{fig:addl_constraints} compares the test accuracy of the LeNet-5 CKN on MNIST when adding additional constraints. As explained in Section~\ref{sec:experiments}, we consider two types of additional constraints. The first type of constraints are generated based on knowledge of whether each unlabeled point has a label in the set $\{4,9\}$ or not. The second type of constraints is randomly generated constraints with approximately the same number of known entries in the adjacency matrix $M$ as for the first type. We can see that both types of additional constraints generally improve the performance of the method. The largest gap occurs when there are 50 labeled observations, as expected. There the accuracies on MNIST when using the additional $\{4,9\}$ constraints and the random constraints are 2\% better and 8\% better, respectively, than without them. This gap shrinks to 0.1\% and 1.4\%, respectively, at 500 observations.
%As noted in Section~\ref{sec:experiments}, it is likely that the better performance with the random constraints than with the $\{4,9\}$ constraints is because the former provide more information to be able to distinguish between labels for often-confused classes.
%%Note that the performance with the $\{4,9\}$ constraints at 150 labels is worse than without the constraints. This is probably because the hold-out validation overfit on the validation set.
%
%\begin{figure}[t]
%\begin{subfigure}{.49\columnwidth}
%\includegraphics[width=1.0\linewidth]{figures/mnist/test_acc_vs_frac_labeled_noerrors_constraints_large.pdf}
%\caption{\label{fig:addl_constraints_mnist} Effect of additional constraints}
%\end{subfigure}\hfill
%\begin{subfigure}{.49\columnwidth}
%\includegraphics[width=1.0\linewidth]{figures/mnist/test_acc_vs_frac_labeled_noerrors_imbalanced_large.pdf}
%\caption{\label{fig:imbalanced data_mnist} Effect of unbalanced data}
%\end{subfigure}
%\caption{\label{fig:addl_constraints} Average accuracy across 10 trials of XSDC after training a LeNet-5 CKN on MNIST when adding additional constraints and varying the fraction of labeled data (left) and when varying the balance of the unlabeled data (right). The ``additional \{4,9\} constraints'' in (a) are derived from knowledge of whether the label for each unlabeled point lies in the set \{4,9\}. The imbalance parameter in (b) denotes the fraction of the labels that are from the set $\{0,1,2,3,4\}$. All classes in the set $\{0,1,2,3,4\}$ are equally represented, and similarly for $\{5,6,7,8,9\}$.}
%\end{figure}
%
%\paragraph{Effect of unbalanced unlabeled data.} Figure~\ref{fig:imbalanced data_mnist} displays the accuracy of the LeNet-5 CKN on MNIST when 50 observations are labeled and the unlabeled data is unbalanced. To make the unlabeled data unbalanced we vary the fraction of the labels $\{0,1,2,3,4\}$ and the fraction of the labels $\{5,6,7,8,9\}$. Within each category 0-4 all of the labels are equally represented, and similarly for 5-9. The imbalance parameter in the plot denotes the fraction of the labels that are from the set $\{0,1,2,3,4\}$.
%
% The performance is generally better when the data is closer to being balanced, as expected. The only time training with the unbalanced data is no better than training on only the labeled data is when 95\% of the unlabeled data is comprised of images of the digits 0-4. At that point the accuracy is on average the same as that of the purely supervised case.

%\paragraph{Sensitivity analysis.}
%Next we perform a sensitivity analysis of the hyperparameters that are tuned via hold-out validation. To be consistent with the other experiments, the setting we choose is when training a LeNet-5 CKN on MNIST with 50 labels. For this architecture the parameters we validate over are the learning rates for the supervised initialization and semi-supervised learning and the penalty on the classifier weights. Here we vary one parameter at a time, fixing all others to their values obtained from hold-out validation (which were $2^{-7}$ and $2^{-6}$ for the learning rates of the supervised initialization and semi-supervised learning, respectively. The penalty on the classifier weights was validated every 100 iterations.). We see that the most important parameter to tune is the semi-supervised learning rate. The other parameters only have a noticeable detrimental effect if they are too large.
%
%
%\begin{figure}[t]
%\begin{subfigure}{.33\columnwidth}
%\includegraphics[width=1.0\linewidth]{figures/sensitivity_analysis/test_acc_vs_labeled_lr.pdf}
%\end{subfigure}\hfill
%\begin{subfigure}{.33\columnwidth}
%\includegraphics[width=1.0\linewidth]{figures/sensitivity_analysis/test_acc_vs_unlabeled_lr.pdf}
%\end{subfigure}
%%\begin{subfigure}{.5\columnwidth}
%%\includegraphics[width=1.0\linewidth]{figures/sensitivity_analysis/test_acc_vs_lambda_pix.pdf}
%%\end{subfigure}
%\begin{subfigure}{0.33\columnwidth}
%\begin{center}
%\includegraphics[width=1.0\linewidth]{figures/sensitivity_analysis/test_acc_vs_lambda.pdf}
%\end{center}
%\end{subfigure}
%\caption{\label{fig:sensitivity} Sensitivity analysis of the hyperparameters tuned with hold-out validation when  using XSDC to train a LeNet-5 CKN on MNIST with 50 labeled observations.}
%\end{figure}


%\paragraph{Comparison to alternative relaxations.} 
%Finally, we compare the convex relaxation of the labeling suproblem presented in Section~\ref{sec:opt} to the relaxation proposed by \citet{bach2007} presented in Appendix~\ref{app:alt_label}. As accomodating constraints on cluster labels is less natural in the latter relaxation, we compare the relaxations when training a LeNet-5 CKN on MNIST with no labeled data. Figure~\ref{fig:relax_comparison} compares our matrix balancing method, the eigendecomposition method from Appendix~\ref{app:alt_label}, and the eigendecomposition method followed by $k$-means clustering. Prior to clustering, the rows of the eigenvector matrix were normalized to have unit $\ell_2$ norm. The value of $\regtwo_0$ was chosen from the set $\{0.01n_b, 0.02n_b,\dots, 0.1n_b\}$, where $n_b$ is the size of a mini-batch, based on the performance on the validation set.
%
%\begin{figure}
%\begin{subfigure}{.49\columnwidth}
%\includegraphics[width=1.0\linewidth]{figures/mnist/mnist_0_alt_labeling_nolambdapix.pdf}
%\caption{\label{fig:relax_comparison_acc} Effect of convex relaxation}
%\end{subfigure}\hfill
%\begin{subfigure}{.49\columnwidth}
%\includegraphics[width=1.0\linewidth]{figures/mnist/mnist_0_eigengap_nolambdapix.pdf}
%\caption{\label{fig:relax_comparison_gap} Evolution of the eigengap}
%\end{subfigure}
%\caption{\label{fig:relax_comparison} Performance of matrix balancing in comparison to eigendecomposition-based methods across 10 trials of training a LeNet-5 CKN on MNIST with no labeled data. The error bands in the plot on the right show one standard deviation from the mean.}
%\end{figure}
%
%From Figure~\ref{fig:relax_comparison_acc} we can see that the convex relaxation used to derive the matrix balancing method is superior to the relaxations leading to the eigendecomposition-based methods. On average, matrix balancing performs 17\% better than the eigendecomposition method and 12\% better than the eigendecomposition method followed by $k$-means. This suggests that the constraint from the convex relaxation requiring the diagonal of $M$ to consist of all $1$'s and/or the constraint requiring all entries of $M$ to be positive are important for the performance of the labeling method.
%
%In Figure~\ref{fig:relax_comparison_gap} we examine the eigengap of $A$ across iterations. The eigengap is defined as $\lambda_{k+1}-\lambda_{k}$, where $k$ is the number of classes and $\lambda_1\leq \dots\leq \lambda_n$ are the eigenvalues of $A$. As noted by \citet{meila2005}, having a larger eigengap makes the subspace spanned by the first $k$ eigenvectors of $A$ more stable to perturbations. From the figure we can see that the eigendecomposition-based methods tend to increase the eigengap as the learning proceeds. For the eigendecomposition method, the eigengap increased from $2\times10^{-6}$ to  $6\times10^{-5}$ on average after 50 iterations. Similarly, for the eigendecomposition method followed by $k$-means, the eigengap increased from  $5\times10^{-6}$ to  $5\times10^{-5}$ on average after 50 iterations. It is interesting to note that matrix balancing, which does not yield low-rank solutions $M^\star$, leads to eigengaps that are extremely small (on the order of $10^{-15}$) across the iterations. Nevertheless, it outperforms the eigendecomposition-based methods.
